# Supplementary material for: Are Neural Nets Modular? Inspecting Functional Modularity Through Differentiable Weight Masks
Source: arXiv:2010.02066 source file (2021-03-06)
Supplement: Supplementary file 1 [file different_notions_of_modularity.tex]

Different authors define modules in different ways. \citet{filan2020neural} defines it as clusters of neurons with strong internal and weak external connectivity, while \citet{watanabe2019interpreting} cluster units hierarchically based on activation statistics. Explicitly modular networks define them by the construction of their architecture. These different modules serve different goals: they may be used to analyze different aspects of a neural network or simply serve as conditional computation units like in routing networks \citep{rosenbaum2019routing}. We are interested in particular types of modules: functional modules that are defined with respect to the function they perform.
This enables us to reason about sharing or specializing computation, which yields interesting insights.
There is no reason to believe however, that these different methods will arrive at the same modules.
For example, if a routing network like the ones by \citet{kirsch2018modular} would be trained on the double-addition task (Section \ref{sec:double_add}), it would undoubtedly use a shared module (by their own definition) because it has no way to process a single input vector by multiple modules.
However, internally these modules might be further divisible by the function of individual weights (our definition), clustering of the connectivity \citep{filan2020neural}, etc.
